# Supplementary material for: Conformational isomerization dynamics in solvent violates both the Stokes-Einstein relation and Kramers' theory
Source: arXiv:2309.07521 ancillary file (2023-09-14)
Supplement: Supplementary file 1 [file SI_Document.pdf]

# Conformational isomerization dynamics in solvent violates both the Stokes-Einstein relation and Kramers' theory - Supplementary Information

Benjamin A. Dalton, Henrik Kiefer, and Roland R. Netz
*Freie Universität Berlin, Fachbereich Physik, 14195 Berlin, Germany*

## CONTENTS

S1. Simulation details and methods 2

S2. Water-glycerol solvent viscosity 3

S3. Position-dependent mass of the butane dihedral 5

S4. The generalised Langevin equation (GLE) and memory kernel extraction 6

S5. Comparison between models with rigid and flexible bond angles 8

S6. Butane translational mean squared displacements 9

S7. Dihedral barrier recrossing 9

S8. Additional information for extended alkane and dipeptide simulations 11

S9. Fitting the viscosity scaling for dihedral barrier-crossing times 13

S10. Kramers' and Grote-Hynes predictions of butane and decane isomerization times 16

S11. Butane dihedral memory kernels and fitting parameters 17

S12. Effects of memory kernel oscillation on Grote-Hynes predictions 19

References 20

## S1. SIMULATION DETAILS AND METHODS

We conducted simulations of single n-alkane molecules and single amino acids in pure water and water-glycerol mixtures to investigate how changes in solvent viscosity affect their behavior. To manipulate the solvent viscosity, we either varied the mass of the water molecules or adjusted the concentration of the co-solvent glycerol.

We carried out all simulations using the GROMACS simulation package (version 2020) and employed the TIP4P/2005 rigid water model [1]. To model glycerol and alkane molecules, we used the GROMOS53A6 force field [2] and represented all n-alkanes as united-atom chains. We neglected non-bonded 1-4 Lennard-Jones interactions and instead included a Ryckaert-Bellemen dihedral potential [3] (discussed below). For glycerol molecules, we explicitly represented all atoms, including hydrogens. We constrained bond lengths using the LINCS constraint algorithm [4]. We allowed all bond angles to vibrate, including the hydrogen atoms in glycerol, except for the case of water. For the amino acid simulations, we studied single alanine and single phenylalanine molecules, each with NMA C-terminal capping and ACE at N-terminal capping, resulting in two dipeptide bonds for each molecule. We used the Amber99 force field, with all bond lengths fixed and all bond angles flexible.

To ensure accurate simulation results, we pre-equilibrate all systems in the NPT ensemble with a Berendsen barostat [5] set to 1 atm. For production runs, we perform all simulations in the NVT ensemble with 2 fs simulation time steps and a temperature of 300 K, controlled with a velocity rescaling thermostat. For butane, we run individual simulations for 10 $\mu$s, which we require for convergence in the long-time-scale memory effects. We analyse data at full-time resolution. For the longer alkane simulations (hexane, octane, and decane), we run individual simulations for 4 $\mu$s and analyse results at a resolution of 20 fs. For the amino acid simulations, we run individual simulations for 3 $\mu$s and analyse results at a full time-resolution. For the calculation of solvent viscosities, we run production simulations for 500 ns. For all production runs, we save trajectories in blocks of 20 ns and analyse each block individually. We then compile the results for each block by averaging. For the mean first-passage times of butane, as shown in Fig. 2 in the main manuscript, we concatenate the 20 ns blocks into blocks of length 500 ns. The error bars in Fig. 2 are standard deviations over 20 blocks of length 500 ns. For amino acid simulations, we exclude events where the $\phi$-dihedral makes a full rotation or enters the rare $\phi = 55$ deg state, as these would require much longer simulations to generate converged trajectories. Any blocks that exhibit these rare events are discarded from the block averaging process.

The butane dihedral is the angle subtended by the intersection of the $CH3_1$-$CH2_2$-$CH2_3$ and the $CH2_2$-$CH2_3$-$CH3_4$ planes. This angle is denoted as $\theta$, where $\theta = 0$ degrees represents the trans-state. The dihedral undergoes transitions between the trans-state, and the two cis-states, located at $\theta = \pm 120$ deg, by overcoming free-energy barriers. The same conventions are used for all longer alkanes. Intra-molecular interactions influence the free-energy profile experienced by the dihedral, and these interactions are included explicitly in a dihedral potential. The large barrier separating the two cis-states can be included via non-bonded 1-4 interactions or by explicitly incorporating the barrier into the dihedral potential function. To prevent cis-to-cis full rotations, we exclude non-bonded interactions and instead include a Ryckaert-Bellemans potential [3]. The Ryckaert-Bellemens potential is expressed as a fifth-order cosine power series: $V_{\mathrm{RB}}(\theta) = \sum_{n=0}^{5} v_n \cos^n(2\pi\theta/360)$, with standard coefficients $v_0 = 9.28$, $v_1 = 12.16$, $v_2 = -13.12$, $v_3 = -3.06$, $v_4 = 26.24$, and $v_5 = -31.50$, in units of $\mathrm{kJmol}^{-1}$. In our simulations of alkanes, no cis-to-cis transitions were observed. For longer alkanes, we use the same dihedral potential with the same parameters for all dihedrals along the chain.

## S2. WATER-GLYCEROL SOLVENT VISCOSITY

For the water-glycerol mixtures, we evaluate the shear viscosity using the equilibrium Green-Kubo relation:

$$\eta_{\mathrm{GK}} = \frac{V}{10 k_{\mathrm{B}} T} \int_0^{\infty} \sum_{\alpha,\beta}^{3} \Big\langle \Pi_{\alpha\beta}(s) \Pi_{\alpha\beta}(s+\tau) \Big\rangle_s d\tau, \tag{S1}$$

where $\Pi_{\alpha\beta}$ is the trace-free stress tensor and $\langle \cdots \rangle_s$ is the ensemble average over $s$. The term inside the integral is the shear stress autocorrelation function (ACF), which we evaluate from MD simulations. In practice, Eq. S1 is a running integral with a finite upper time limit. For improved statistics, we average over $N_{\mathrm{T}}$ individual trajectories. For individual trajectories, the finite-time running integral approximation of Eq. S1 is:

$$I_j(t) = \frac{V}{10 k_{\mathrm{B}} T} \int_0^{t} \sum_{\alpha,\beta}^{3} \Big\langle \Pi_{\alpha\beta,j}(0) \Pi_{\alpha\beta,j}(\tau) \Big\rangle d\tau, \tag{S2}$$

where $j = 1, 2, ..., N_{\mathrm{T}}$. The average running integral is then:

$$I(t) = \frac{1}{N_{\mathrm{T}}} \sum_{j=1}^{N_{\mathrm{T}}} I_j(t). \tag{S3}$$

In Fig. S1A, we show the ensemble-averaged running integral $I(t)$ for pure water in atmospheric conditions with standard mass. We show the $I_j(t)$ from individual trajectories in blue with the result from Eq. S3 in black. On average, the stress ACFs decay after approximately 5 ps. However, the individual integrals are scattered. We select a plateau region, between the bounds of $t_{\mathrm{min}}$ and $t_{\mathrm{max}}$, where Eq. S3 is well converged, and we approximate the solvent viscosity as the average of $I(t)$ in this region:

$$\eta = \frac{1}{t_{\mathrm{max}} - t_{\mathrm{min}}} \int_{t_{\mathrm{min}}}^{t_{\mathrm{max}}} I(t) dt. \tag{S4}$$

The red overlay in Fig. S1A indicates the selected plateau region. We perform this calculation for all water-glycerol

TABLE S1. Compositions of water-glycerol mixtures, indicating the number of water molecules $N_{\mathrm{w}}$ and the number of glycerol molecules $N_{\mathrm{gly}}$ for each mixture. The concentrations of glycerol are given as the mass percentages.

| % glycerol | $N_{\mathrm{w}}$ | $N_{\mathrm{gly}}$ | $\eta$ [mPa · s] | $\eta/\eta_0$ |
|---|---|---|---|---|
| 0 | 1500 | 0 | 0.86 | 1.0 |
| 10 | 1350 | 29 | 1.11 | 1.3 |
| 20 | 1200 | 59 | 1.54 | 1.8 |
| 30 | 1050 | 88 | 2.20 | 2.5 |
| 40 | 900 | 117 | 3.42 | 3.9 |
| 50 | 750 | 147 | 5.80 | 6.7 |
| 60 | 600 | 176 | 12.16 | 14.0 |

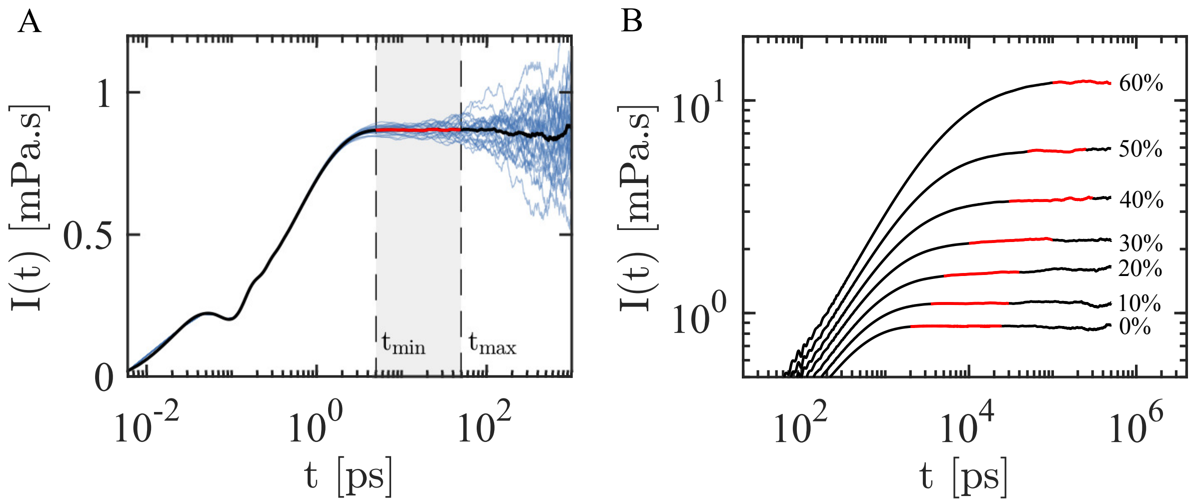


FIG. S1. Calculating viscosity for water-glycerol mixtures with the Green-Kubo method. (A) Running integral of stress ACF for pure water, according to Eq. S3. The black curve is the average of 25 trajectories. The individual trajectories are shown in blue. The plateau region (red overlay) is set by choosing the bounds $t_{min}$ and $t_{max}$. (B) The average running integrals for the range of glycerol concentrations, with the chosen plateau regions (shown in red).

solvent compositions. The numerical results are presented in Table S1. In Fig. S1B, we show Eq. S3 for each composition, with plateau regions indicated in red.

We plot the results for Eq. S3 in Fig. 1E of the main text, where we show good agreement with experimental results.

## S3. POSITION-DEPENDENT MASS OF THE BUTANE DIHEDRAL

In the main manuscript, we treat the effective mass of all dihedrals to be constant. This is an approximation. It is known that the rigid butane model, introduced in Section S5, exhibits position-dependent mass [6]. This is important when considering the position dependence of the friction memory kernel, which we neglect in this paper. Regardless, in Fig. S2, we show that the mass for the flexible butane model used throughout this paper also depends on the position, which we calculate using histograms for the position-dependent dihedral velocity $\dot{\theta}(\theta)$, and hence the position-dependent equipartition theorem $m_{\text{eff}}(\theta) = k_{\text{B}}T/\langle\dot{\theta}(\theta)\rangle^2$. The values used for the constant mass are indicated in the figure. Note that in the main manuscript and all other sections of this SI, the effective, position-independent mass is simply denoted $m$.

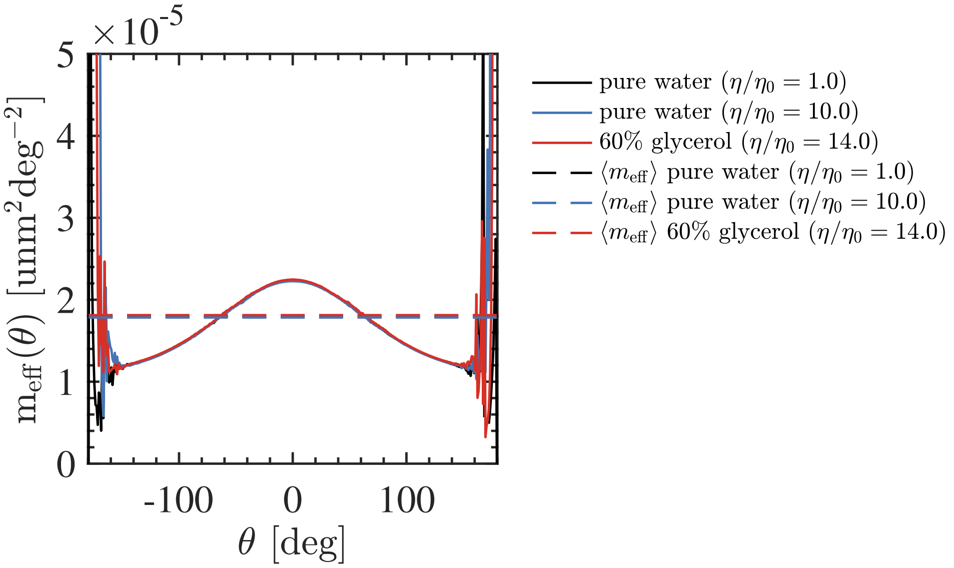


FIG. S2. Effective mass profiles for the butane dihedral, evaluated over a range of solvent viscosity conditions. The profiles are evaluated using a position-dependent equipartition theorem $m_{\text{eff}}(\theta) = k_{\text{B}}T/\langle\dot{\theta}(\theta)\rangle^2$. The dashed lines show the position-independent mean values used throughout the main manuscript.

## S4. THE GENERALISED LANGEVIN EQUATION (GLE) AND MEMORY KERNEL EXTRACTION

All MD simulation trajectories are projected onto a dihedral-angle reaction coordinate $\theta(t)$, which we map onto a 1D GLE:

$$m\ddot{\theta}(t) = -\int\limits_0^t \Gamma(t-t')\dot{\theta}(t')dt' - \frac{\partial}{\partial\theta}U\big[\theta(t)\big] + F_R(t), \tag{S5}$$

where we exclude any position dependence of the memory kernel [6]. $F_R(t)$ is the random force term, which has a zero mean $\langle F_R(t)\rangle = 0$, and satisfies the fluctuation-dissipation theorem $\langle F_R(t)F_R(t')\rangle = k_\mathrm{B}T\Gamma(t-t')$. $U(\theta)$ is the potential of mean force, which is extracted uniquely for each system according to $U(\theta) = -k_\mathrm{B}T\log\big[\rho(\theta)\big]$, where $\rho(\theta)$ is the probability density over $\theta(t)$. The total friction on the dihedral is given by the converged plateau value of the integrated memory kernel:

$$\gamma = G(t\to\infty) = \int_0^\infty \Gamma(t)dt, \tag{S6}$$

where $G(t) = \int_0^t \Gamma(t')dt'$ is the running integral of the memory kernel.

To extract $\Gamma(t)$, we use the running integral extraction scheme in the presence of general potentials [7, 8]. We correlate Eq. S5 with the initial position of the dihedral angle $\theta(0)$:

$$m\Big\langle\theta(0)\ddot{\theta}(t)\Big\rangle = -\int\limits_0^t \Gamma(t-t')\Big\langle\theta(0)\dot{\theta}(t')dt'\Big\rangle - \Big\langle\theta(0)\nabla U\big[\theta(t)\big]\Big\rangle + \Big\langle\theta(0)F_R(t)\Big\rangle, \tag{S7}$$

and with the initial velocity of the dihedral angle $\dot{\theta}(0)$:

$$m\Big\langle\dot{\theta}(0)\ddot{\theta}(t)\Big\rangle = -\int\limits_0^t \Gamma(t-t')\Big\langle\dot{\theta}(0)\dot{\theta}(t')dt'\Big\rangle - \Big\langle\dot{\theta}(0)\nabla U\big[\theta(t)\big]\Big\rangle + \Big\langle\dot{\theta}(0)F_R(t)\Big\rangle, \tag{S8}$$

Due to the original orthogonality relations used to derive the GLE in Eq. S5, both $\big\langle\theta(0)F_R(t)\big\rangle = 0$ and $\big\langle\dot{\theta}(0)F_R(t)\big\rangle = 0$. We write Eqs. S7 and S8 in terms of the position-velocity and velocity-velocity correlation functions $C^{\theta\dot{\theta}}(t) = \big\langle\theta(0)\dot{\theta}(t)\big\rangle$ and $C^{\dot{\theta}\dot{\theta}}(t) = \big\langle\dot{\theta}(0)\dot{\theta}(t)\big\rangle$, respectively, as well as the correlations between the dihedral angle and the PMF gradients $C^{\theta\nabla U}(t) = \big\langle\theta(0)\nabla U\big[\theta(t)\big]\big\rangle$, and the velocity of the dihedral angle and the PMF gradients $C^{\theta\nabla U}(t) = \big\langle\dot{\theta}(0)\nabla U\big[\theta(t)\big]\big\rangle$:

$$m\frac{d}{dt}C^{\theta\dot{\theta}}(t) = -\int_0^t \Gamma(t')C^{\theta\dot{\theta}}(t-t')dt' - C^{\theta\nabla U}(t), \tag{S9}$$

$$m\frac{d}{dt}C^{\dot{\theta}\dot{\theta}}(t) = -\int_0^t \Gamma(t')C^{\dot{\theta}\dot{\theta}}(t-t')dt' - C^{\dot{\theta}\nabla U}(t). \tag{S10}$$

We integrate Eq. S10 in the time domain and obtain an equation in terms of $G(t) = \int_0^t \Gamma(t')dt'$:

$$mC^{\dot{\theta}\dot{\theta}}(t) - mC^{\dot{\theta}\dot{\theta}}(0) = -\int_0^t G(t-t')C^{\dot{\theta}\dot{\theta}}(t'')dt'' + C^{\theta\nabla U}(t) - C^{\theta\nabla U}(0). \tag{S11}$$

Using the identity $\frac{d}{dt}C^{\theta\dot{\theta}}(t) = C^{\theta\ddot{\theta}}(t) = -C^{\dot{\theta}\dot{\theta}}(t)$, we evaluate Eq. S9 at t=0, and obtain $mC^{\dot{\theta}\dot{\theta}}(0) = C^{\theta\nabla U}(0)$. It follows that:

$$\frac{C^{\dot{\theta}\dot{\theta}}(t)}{C^{\dot{\theta}\dot{\theta}}(0)}C^{\theta\nabla U}(0) = C^{\theta\nabla U}(t) - \int_0^t G(t-t')C^{\dot{\theta}\dot{\theta}}(t'')dt''. \tag{S12}$$

Eq. S12 can be discretized using the trapezoidal rule for numerical integration. Using $G(0) = 0$, we arrive at the following numerical extraction scheme, which we use to extract the discrete representation of $G(t)$ directly from the trajectory of a given dihedral angle:

$$G_i = \begin{cases} 0, & i = 0 \\ \frac{2}{\Delta t C_0^{\dot\theta\dot\theta}}\left[C_1^{\nabla U\theta} - \frac{C_0^{\nabla U\theta}}{C_0^{\dot\theta\dot\theta}} C_1^{\dot\theta\dot\theta}\right], & i = 1 \\ \frac{2}{\Delta t C_0^{\dot\theta\dot\theta}}\left[C_i^{\nabla U\theta} - \frac{C_0^{\nabla U\theta}}{C_0^{\dot\theta\dot\theta}} C_i^{\dot\theta\dot\theta} - \Delta t \sum_{j=1}^{i-1} G_j C_{i-j}^{\dot\theta\dot\theta}\right], & i > 1 \end{cases} \tag{S13}$$

where $C_i^{\dot\theta\dot\theta}$ and $C_i^{\nabla U\theta}$ are the discretized representations of the velocity-velocity correlation function and the correlations between the dihedral angle and the gradients of the PMF, respectively.

## S5. COMPARISON BETWEEN MODELS WITH RIGID AND FLEXIBLE BOND ANGLES

Here, we compare results from the butane model used in the main manuscript, which has flexible bond angles, to two alternative models, both which have rigidly constrained bond angles.

In Fig. S3A, we show normalised memory kernels for butane with flexible bond angles (same as Fig.2B of the main manuscript) and for butane with rigid bond angles. Here, both models exclude non-bonded interactions between the 1-4 CH groups. For both systems, the dihedral free energy profile is fully accounted for by a Ryckaert-Bellemen potential, as discussed in section S1. The aim is to show the contributions to the memory kernel due to the inclusion of oscillating bond angle degrees of freedom.

In Fig. S3B-C, we show the mean first-passage times ($\tau_{\mathrm{MFP}}$) and total friction ($\gamma$) for butane with flexible bond angles (same as main manuscript) and for a butane model with rigidly constrained bond angles and included non-bonded interactions between the 1-4 CH groups. This rigid model is the same model used by Daldrop et. al [9]. The non-bonded 1-4 interactions prevent cis-to-cis transitions. To include isomerization barriers, a periodic potential with of the form $A(1+\cos(2\pi n/360))$, where $n=3$ and $A=5.9$ kJmol$^{-1}$, is used in place of a Ryckaert-Bellemen dihedral potential. In Fig. S3C, where we compare the total friction on the dihedral, we also explicitly show the results from [9], where the low viscosity regime ($\eta/\eta_0 = 0.1$ and 0.3) was also investigated. We note that for $\eta/\eta_0 \geq 1.0$, all models exhibit approximate $(\eta/\eta_0)^{0.4}$ scaling.

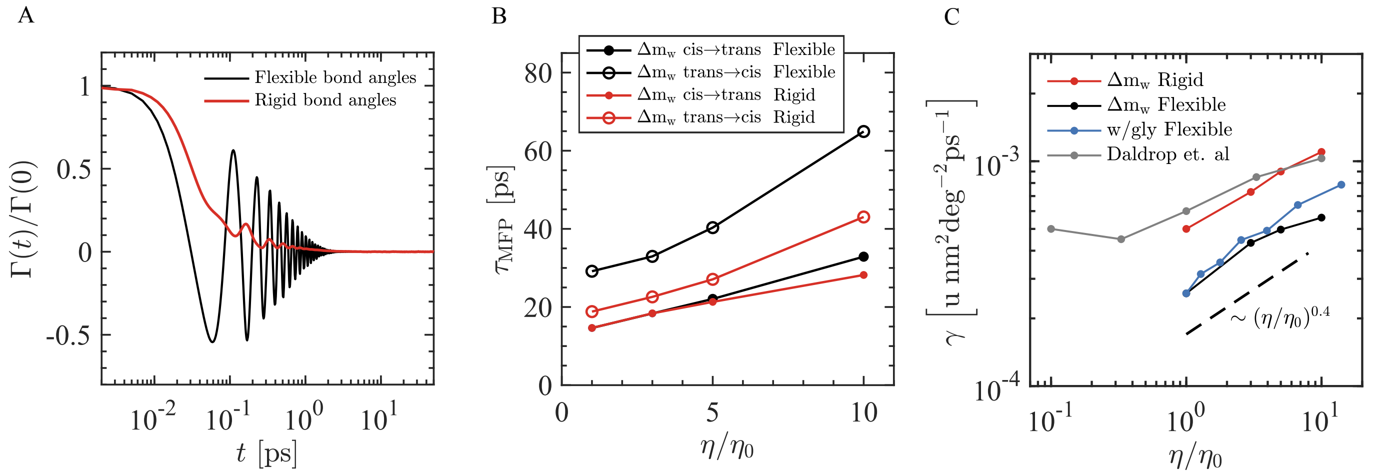


FIG. S3. Comparison of memory kernels and barrier crossing times for butane molecules with flexible and rigidly constrained bond angles. A) Memory kernels for butane simulated in pure water with standard water mass ($\eta/\eta_0 = 1$). Both molecules have a Ryckaert-Bellemen dihedral potential and excluded non-bonded 1-4 interactions. The rigid butane is constrained using the SHAKE algorithm [10]. While the memory kernel for the rigid model exhibits weak oscillating modes, the flexible bond molecule has strongly oscillating memory effects in the dihedral dynamics. Note that both models have rigidly constrained bond lengths. For all data in the main text we use the flexible bond-angle model. B) Barrier crossing times for butane super-heavy water, plotted as a function of viscosity. The black data points are the same as those shown in Fig. 2 of the main manuscript for the super-heavy water systems (flexible bond angles). Red data points are generated using the same model as Daldrop *et. al.* [9], where the bond angles and lengths are rigidly constrained. C) Comparison of total friction $\gamma$ for the flexible and rigid butane models. Results presented by Daldrop et. al [9] are also explicitly shown, which includes results for $\eta/\eta_0 < 1$. For $\eta/\eta_0 \geq 1$, all systems exhibit approximately $(\eta/\eta_0)^{0.4}$ scaling.

## S6. BUTANE TRANSLATIONAL MEAN SQUARED DISPLACEMENTS

The translational diffusion coefficients for the butane centre of mass, as shown in Fig. 2C of the main text, are determined by fitting the long-time diffusive regime for the centre of mass mean squared displacements (MSD). We show the MSDs for all solvent conditions in Fig. S4, and we indicate the long-time diffusive regimes in red, which are approximately linear (compare to the linear scaling lines on each figure). The MSDs are evaluated using the *gmx msd* GROMACS library. The diffusion coefficient is given by the gradient of a linear fit and we normalise using $D_0$, which is the diffusion coefficient for the 0% glycerol, or $m/m = 1$, system.

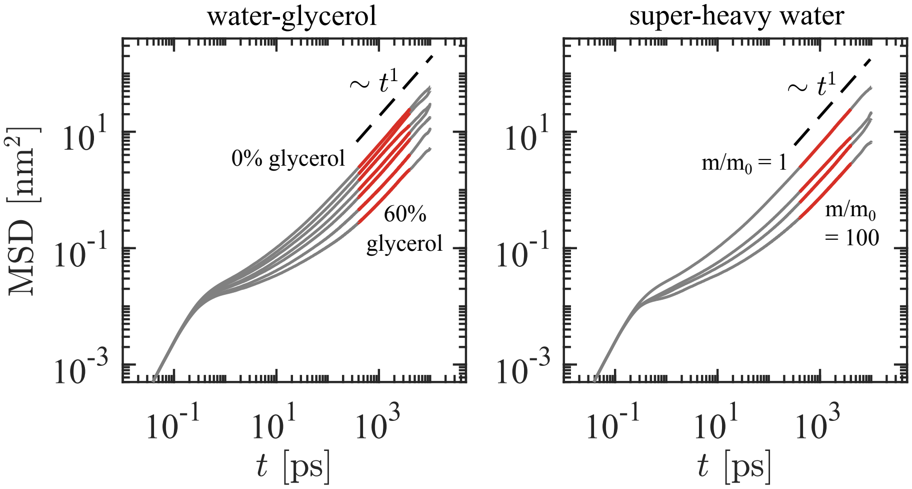


FIG. S4. Mean squared displacements (MSD) for the butane centre of mass translational diffusion. For the water-glycerol system, the 0% glycerol and 60% glycerol curves are indicated. The MSDs for the remaining concentrations are organised monotonically between these two extremes. The same is true for the super-heavy water system, where we indicate the lowest and highest viscosity systems, $m/m = 1$ and 100, respectively. The long-time diffusive regimes are indicated in red for each MSD. The black dashed lines show linear scaling.

## S7. DIHEDRAL BARRIER RECROSSING

Butane exhibits significant recrossing behaviour where, upon entering a new state, the dihedral can either quickly move to a neighbouring state or remain in the current state briefly before transitioning again. In Fig. S5A, we show a short trajectory segment for a butane dihedral in super-heavy water with $\eta/\eta_0 = 10.0$ which displays multiple instances of immediate recrossing and multiple brief state residencies. In Fig. S5B, we show various definitions of barrier crossing times and we construct a distribution for each definition. $\tau_{\mathrm{AFP}}$, as indicated along the top of the figure, shows five examples of sequential all-to-first passage (AFP) times. The all-to-first passage times account for each crossing of the trans-state before crossing into the cis-state. The time interval between consecutive crossings within a single state and the first crossing into the subsequent state are the events that contribute to the all-to-first passage time distribution. The single $\tau_{\mathrm{FFP}}$ shown in Fig. S5B is an example of a first-to-first passage (FFP) event, defined as the first crossing into a new state while disregarding any subsequent crossings. The complete series of $\tau_{\mathrm{FFP}}$ durations obtained throughout a trajectory is used to calculate the mean first-first passage time distribution. To compile a distribution of crossing times that neglects recrossing events, we introduce a delay time $\delta t$. When entering a new state, any crossings occurring during the initial period are discarded until a chosen delay time, represented by $\delta t$, has passed. Once the delay time has elapsed, all subsequent crossing times $\tau_{\mathrm{DAFP}}$ are compiled into a distribution. This process results in the mean delayed all-first passage (DAFP) time distribution and the definition of $\tau_{\mathrm{MPT}}$ that appears in the main text is the mean value of this distribution. In this way, the introduced delay time ensures that the mean of the accumulated distribution represents the distribution in the absence of recrossing. In the absence of recrossing dynamics, the distribution of crossing times is exponential. Since the distribution is normalized, introducing the delay time only affects the amplitude of the recrossing-free contribution and not the mean.

The signatures of recrossing are evident in Figs. S5C - E. Specifically, Figs. S5C and D illustrate the distribution of first-first crossing times ($\tau_{\mathrm{FFP}}$) observed in long butane trajectories for both standard water solvent and the highest

mass super-heavy water solvent. Fig. S5D, which is the same data as B presented on a log plot, shows the results of fitting single-component exponential functions to the distributions for times greater than 10 and 33 ps, respectively. The inset of Fig. S5C also shows deviations from a single component exponential distribution at short times for the standard water mass system. These deviations suggest that recrossing dynamics are present. We further illustrate this in Fig. S5E, where we show distributions for the number of times that a dihedral crosses the trans-state before transitioning to a neighbouring cis-state. For example, in the schematic shown in Fig. S5B, there are 5 crossings of the trans-state before transitioning to the cis-state. In the standard water system, the distribution for the number of crossings is dominated by small numbers. In the high viscosity system, the distribution is characterized by the onset of many decaying exponential modes, similar to the crossing time distribution shown in Fig. S5D. Together, Figs. S5C - E demonstrate that recrossing dynamics significantly impact the kinetics of butane isomerization.

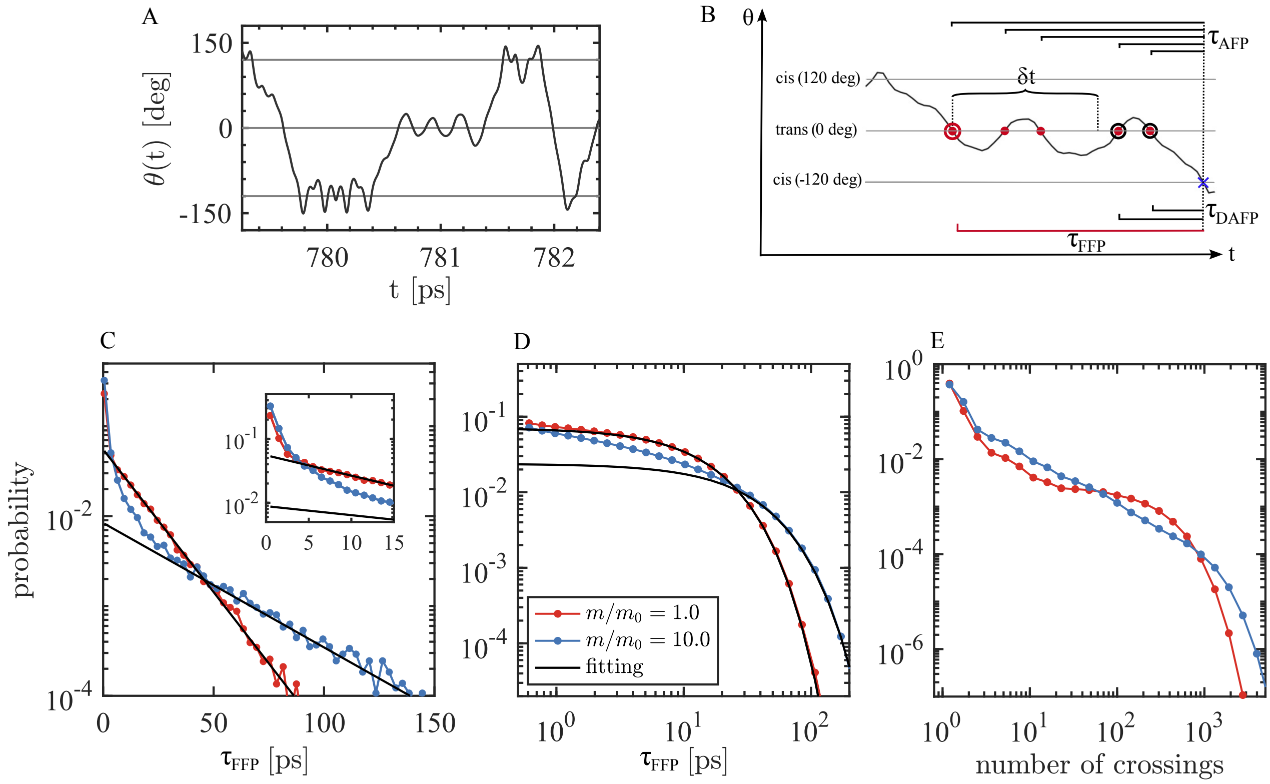


FIG. S5. A) A short trajectory segment showing a combination of recrossing events and short residencies. B) An example trajectory segment showing the butane dihedral as it passes through 3 isomeric-states. The red points show dihedral crossings over the trans-state minimum. The open red circle shows the first crossing into the trans-state minimum, and the blue cross shows the first crossing to the subsequent cis-state minimum. The black circles show the crossings of the trans-state minimum that occur later than $\delta t$. The black lines at the top of the figure show all of the first-passage times from each crossing of the trans-state minimum to the first arrival in the cis-state (here there are 5) for this example transition. This is the set of all-to-first passage events. The red line at the bottom shows the transition time for the first-to-first passage. The two black lines at the bottom show all of the passage times from the trans to the cis-state after $\delta t$ for this example transition. These are the delayed-all-to-first events. C) Distributions of first-to-first passage times taken over a long butane trajectoy (total time 2 $\mu$s) for trans-to-cis transitions. We accumulate the distributions using equally separated histogram bins, suitable for plotting on a linear scale for the crossing times. Single-component exponentials are fit to the long-time tails of the distributions. D) Distributions of first-to-first passage times accumulated in histograms with exponentially increasing bin widths, suitable for plotting on a logarithmic scale. Single-component exponentials are fit to the long-time tails of the distributions. Deviations at short times indicate recrossing contributions. E) Distributions for the number of times a butane dihedral crosses the trans-state before transitioning back to either cis-state. We accumulate the distributions in histograms with exponentially increasing bin widths.

## S8. ADDITIONAL INFORMATION FOR EXTENDED ALKANE AND DIPEPTIDE SIMULATIONS

For all alkane chains, we exclude non-bonded 1-4 Lennard-Jones interactions and hence include the Ryckaert-Bellemen dihedral potentials. In Fig. S6, we show the free energy profiles, extracted from MD simulations, for the inner-most (left) and outer-most (right) dihedrals, as described in Fig. 5A of the main document. We see that all free energy profiles are effectively equivalent, except for the case of butane and the set of outer dihedrals. For butane, the 1st and 4th carbon-hydrogen groups are both CH3 groups. Thus, the united-atom sequence along the dihedral is CH3-CH2-CH2-CH3. For all other chains, the outer-most group resides in a sequence CH3-CH2-CH2-CH2. There is no reason to expect identical solvation contributions around the different sequences. For the inner dihedral, the free energy barrier height in the trans-state is 5.02 $k_\mathrm{B}T$ for butane and 5.1 $k_\mathrm{B}T$ for all other alkanes. In the cis-state, it is 3.9 $k_\mathrm{B}T$ for butane and 3.8 $k_\mathrm{B}T$ for all other alkanes. For the outer dihedral, the hexane, octane, and decane have slightly larger barrier heights in the trans-state of 5.2 $k_\mathrm{B}T$, and cis-state barrier heights of 3.6 $k_\mathrm{B}T$. Overall, the free energy deviations are small ($\mathrm{e}^{5.2}/\mathrm{e}^{5.02} = 1.2$) and do not significantly influence barrier crossing times.

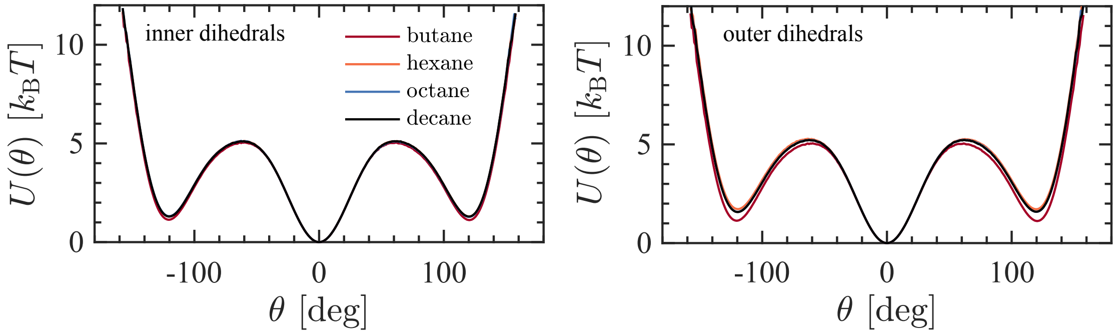


FIG. S6. Free energy profiles for the inner and outer dihedrals of various alkane chains. All dihedral potentials are included using Ryckaert-Bellemen potentials.

Additionally, we show the viscosity-dependence of the $\tau_\mathrm{MFP}$ scaling along the sequence of dihedrals in the decane molecule. The chain containing 7 dihedrals is symmetric around the 4th dihedral (Fig. S7A.) In Fig. S7B, we can see that the different dihedrals exhibit slightly different barrier-crossing scaling. Regardless, the scaling for the two different solvent types diverges for all dihedrals between $\eta/\eta_0 = 3$ and 5.

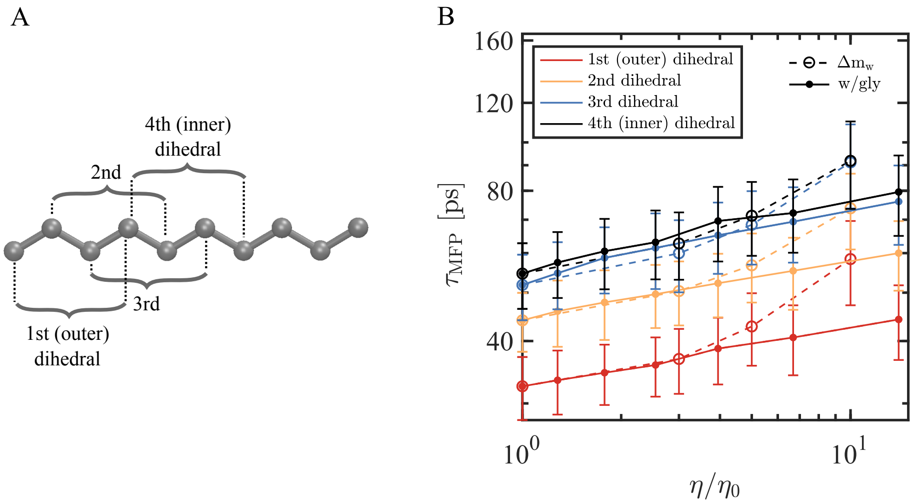


FIG. S7. Viscosity scaling of the decane dihedral barrier-crossing times. A) Location of dihedrals. The chain is symmetric around the 4th (inner) dihedral. Only the 1st, 2nd, 3rd, and 4th locations are indicated. B) Barrier crossing times as a function of viscosity for the set of dihedrals in the two different solvent types.

In the inset of Fig. 3C in the main manuscript, we see that the phenylalanine barrier height ($\Delta U = 2.3\ k_\mathrm{B}$T) is 20% higher than the alanine barrier ($\Delta U = 1.8\ k_\mathrm{B}$T). To approximate whether the increase of $\tau^0_\mathrm{MFP}$ is due to the

change in barrier height, we use a simple Arrhenius model assuming that changes in the relevant curvatures of the free-energy profile are negligible. For alanine in standard water $\tau^0_{\rm MFP} = A{\rm e}^{1.8} = 11.7$ ps, such that $A = 1.93$ ps. If the increase in $\tau^0_{\rm MFP}$ is entirely due to changes in $U$, then for phenylalanine, we should expect $\tau^0_{\rm MFP} = 1.93{\rm e}^{2.3} = 19.1$ ps, which is 40% below the measured value.

## S9. FITTING THE VISCOSITY SCALING FOR DIHEDRAL BARRIER-CROSSING TIMES

The viscosity scaling of the barrier-crossing times for all molecules is fitted to a power law scaling: $\tau_{\mathrm{MFP}}(\eta/\eta_0) = \alpha(\eta/\eta_0)^{\beta} + \varepsilon$. The results for $\alpha$, $\beta$, and $\varepsilon$, as used in Fig. 5E of the main manuscript, are obtained by fits to the $\tau_{\mathrm{MFP}}$ values, as measured in the simulation. We include two constraints on the fitting: $\beta \leq 1$ and $\varepsilon \geq 0$. In Fig. S8, we show the $\tau_{\mathrm{MFP}}(\eta/\eta_0)$ for the inner-most dihedral over all alkanes, and the fits. In Fig. S9, we show the viscosity scaling for the outer-most dihedral (same data as in Fig. S7). The viscosity scaling and subsequent fitting for the alanine and phenylalanine are also shown (Fig. S10). Note that for the alkane inner dihedrals, for the case of butane and hexane in the super-heavy water solvent (Figs. S8A and B), we only fit $\eta/\eta_0 = 3, 5, 10$. This scaling is known to be linear in the high-viscosity regimes [9], but is dominated by internal friction in the low viscosity regime. We neglect the first data point $\eta/\eta_0 = 1$ to avoid including the internal-friction-dominated regime, for which we would obtain $\beta > 1$.

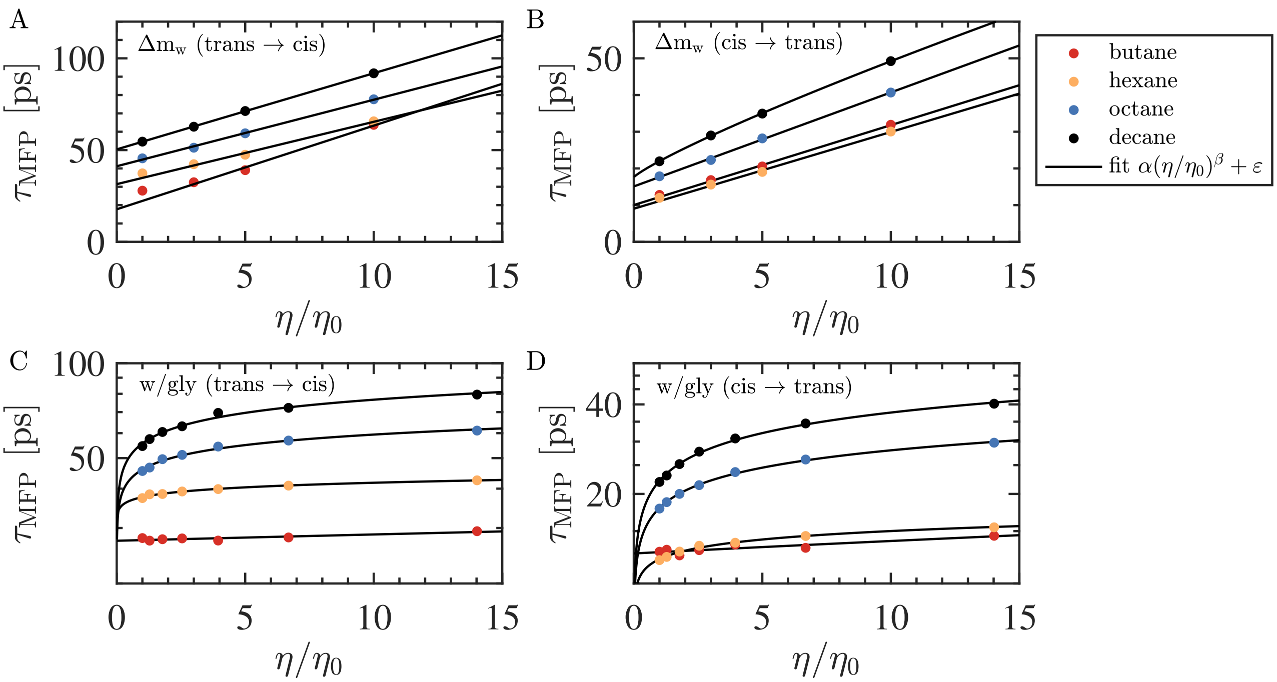


FIG. S8. Viscosity scaling of $\tau_{\mathrm{MFP}}$ for the inner-most dihedral of the four alkanes. Coloured points are simulation data. The black lines are fits to $\tau_{\mathrm{MFP}}(\eta/\eta_0) = \alpha(\eta/\eta_0)^{\beta} + \varepsilon$.

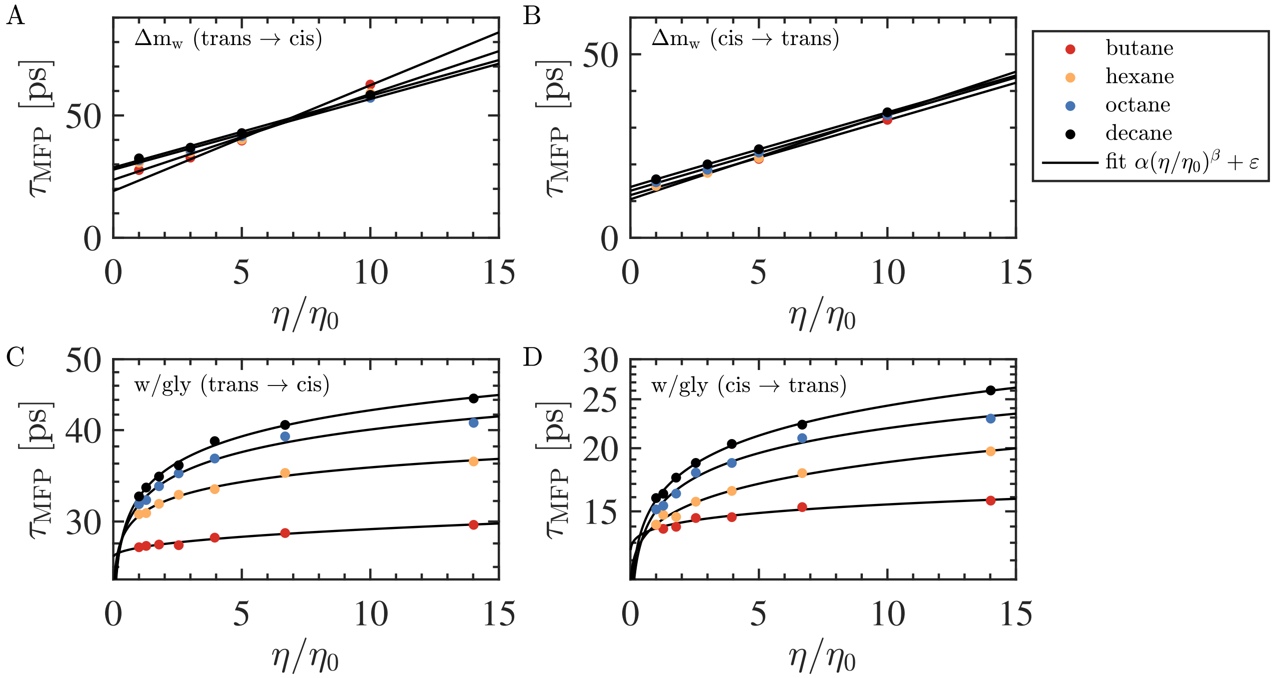


FIG. S9. Viscosity scaling of $\tau_{\mathrm{MFP}}$ for the outer-most dihedral for the four alkanes. Coloured points are simulation data. The black solid lines are fits to $\tau_{\mathrm{MFP}}(\eta/\eta_0) = \alpha(\eta/\eta_0)^{\beta} + \varepsilon$.

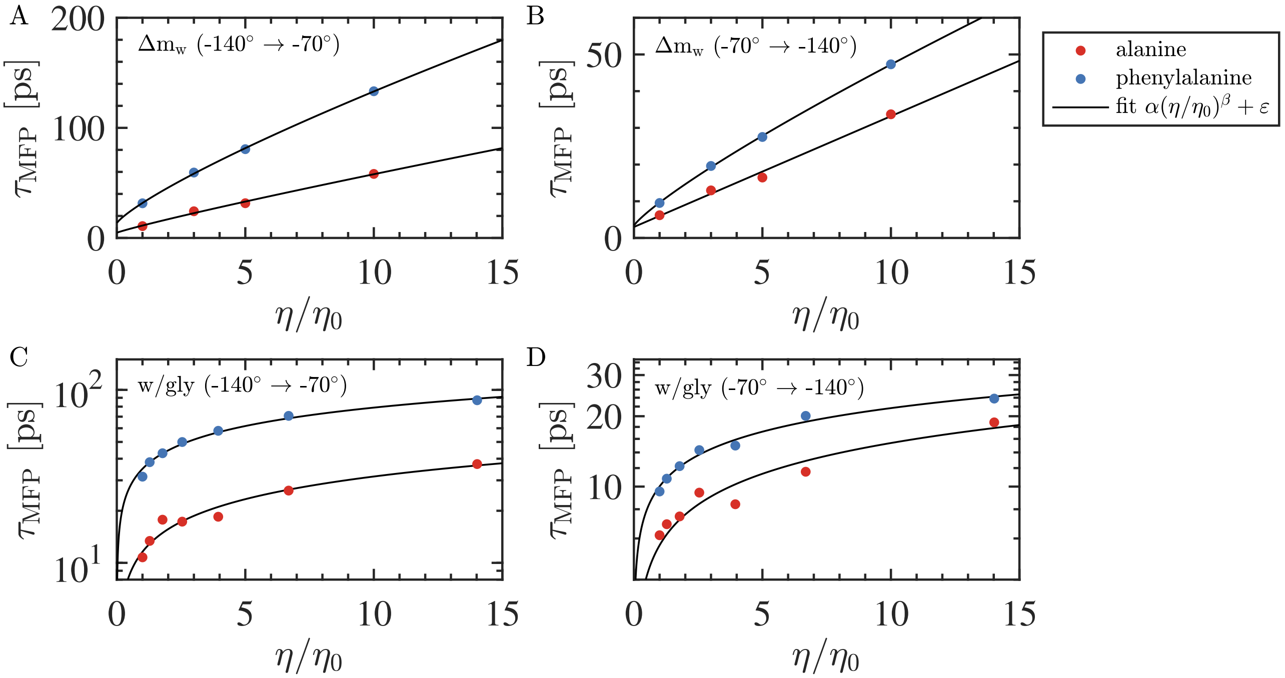


FIG. S10. Viscosity scaling of $\tau_{\mathrm{MFP}}$ for the $\phi$-dihedral for the capped alanine and phenylalanine amino acids. Coloured points are simulation data. The black lines are fits to $\tau_{\mathrm{MFP}}(\eta/\eta_0) = \alpha(\eta/\eta_0)^{\beta} + \varepsilon$.

In Figs. S11 and S12, we show the full set of parameters obtained by fitting the viscosity scaling for the inner-most alkane dihedrals and the two capped amino-acids. The results for $\beta$ and $\varepsilon/(\alpha+\varepsilon)$ are shown in the main manuscript.

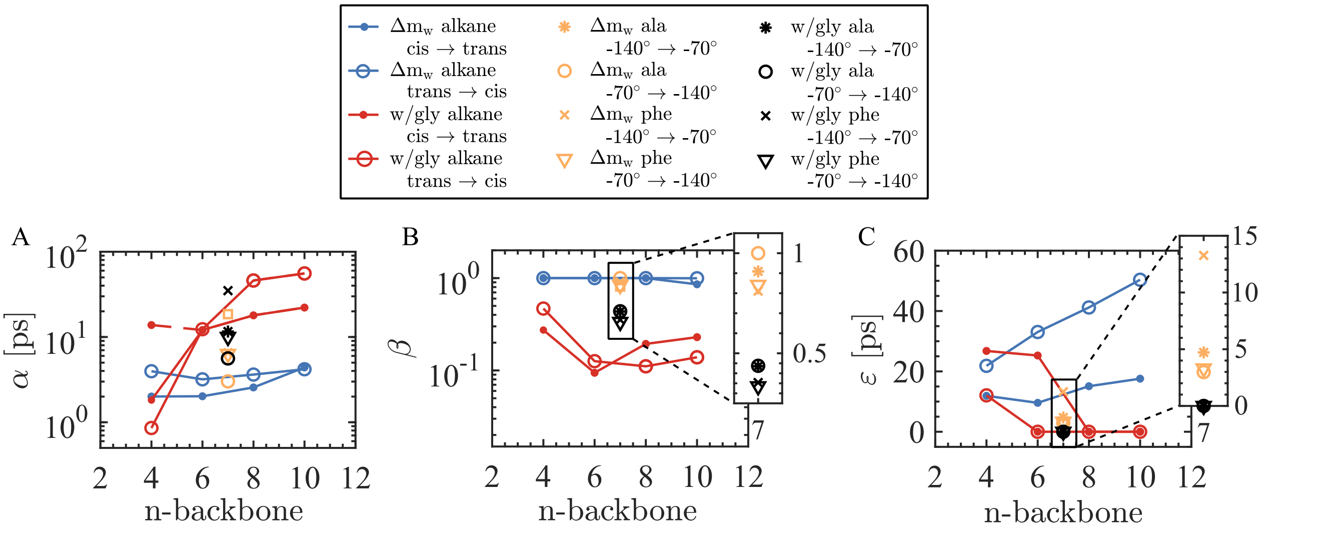


FIG. S11. Fitting parameters for the alkane inner-most dihedrals, and for the amino acid $\phi$ dihedrals. For the alkanes, the parameters are plotted as a function of the alkane chain length, where the carbon atoms are considered as the back-bone. For the amino acids, there is only a single backbone length. The insets for B) and C) show the magnification for the amino acid values from the main panel.

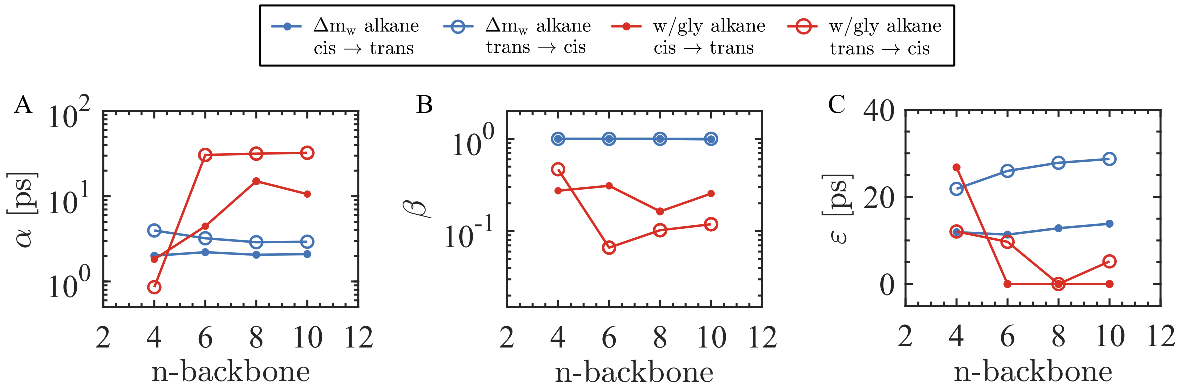


FIG. S12. Fitting parameters for the alkane outer-most dihedrals.

## S10. KRAMERS' AND GROTE-HYNES PREDICTIONS OF BUTANE AND DECANE ISOMERIZATION TIMES

Since we directly extract the friction acting on the rotating dihedral, we can evaluate various reaction-rate theory predictions for the dihedral transition times and compare to the simulation results in Fig. 3B in the main manuscript. The Grote-Hynes prediction for barrier crossing with frequency-dependent friction is given by [11]

$$\tau_{\rm GH} = \frac{2\pi\omega_{\rm max}}{\lambda\omega_{\rm min}} {\rm e}^{\beta U_0}, \tag{S14}$$

where $\omega_{\rm max} = \sqrt{|U''_{\rm max}|/m}$ and $\omega_{\rm min} = \sqrt{U''_{\rm min}/m}$ are the barrier frequencies at the free energy maximum and minimum, with curvatures $U''_{\rm max}$ and $U''_{\rm min}$. $m$ is the effective mass of the dihedral, here taken to be constant, given by the equipartition theorem $m = k_{\rm B}T/\langle\dot\theta\rangle^2$. For the cis→trans transition in butane, $|U''_{\rm max}| = 1.35\times10^{-3}\ k_{\rm B}T/{\rm deg}^2$ and $U''_{\rm min} = 6.25\times10^{-3}\ k_{\rm B}T/{\rm deg}^2$, with a barrier height $U_0 = 3.9\ k_{\rm B}T$. $\lambda$ is the barrier reactive frequency determined by solving the Grote-Hynes equation

$$m\lambda^2 + \lambda\tilde\Gamma(\lambda) - m\omega_{\rm max}^2 = 0, \tag{S15}$$

where $\tilde\Gamma(\lambda)$ is the Laplace transform of the friction memory kernel, given by $\tilde\Gamma(\lambda) = \int_0^\infty \Gamma(t'){\rm e}^{-\lambda t'}dt'$, which we evaluate numerically. In the Markovian limit, i.e. when $\Gamma(t) = \gamma\delta(t)$, Eq. S14 reduces to the well-known Kramers prediction

$$\tau_{\rm Kr} = \left[\sqrt{\frac{\gamma^2}{4m^2} + \omega_{\rm max}^2} - \frac{\gamma}{2m}\right]^{-1} \frac{2\pi\omega_{\rm max}}{\omega_{\rm min}} {\rm e}^{\beta U_0}. \tag{S16}$$

In Fig. S13, we see that neither the Grote-Hynes, nor the Kramers theory, can consistently predict the viscosity scaling of $\tau_{\rm MFP}$ for both butane and the decane inner dihedral, in both the super-heavy water and water-glycerol mixture. In particular, neither theory is able to predict the strongly disparate behaviour for the butane $\tau_{\rm MFP}$, as present in Fig. 2D of the main manuscript. It is not surprising that the Kramers prediction does not represent the simulation data well since it is suitable for Markovian systems. The Grote-Hynes theory, however, explicitly incorporates non-Markovian effects. The breakdown of the Grote-Hynes theory in the small molecule regime indicates complex non-Markovian effects that the Grote-Hynes theory cannot capture.

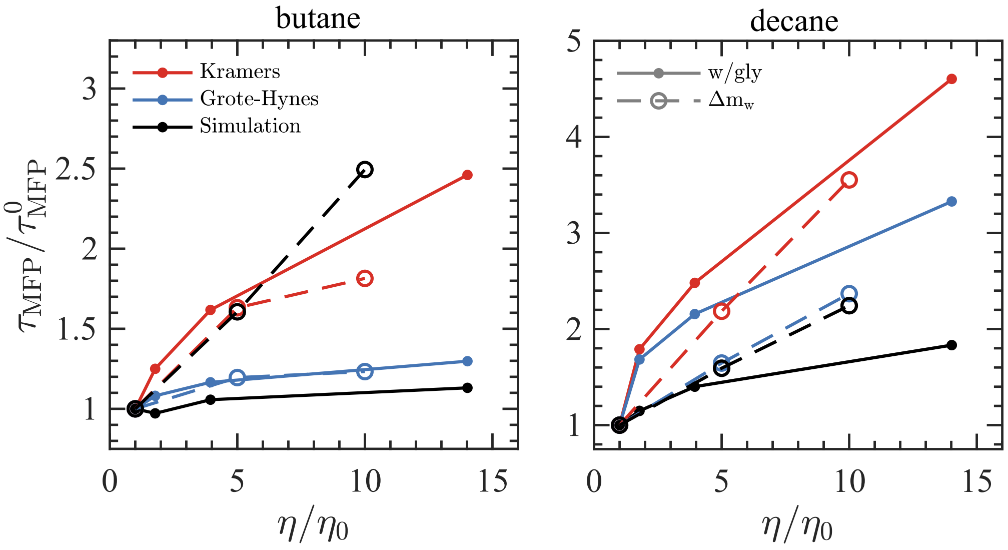


FIG. S13. Comparison of the Kramers prediction (Eq. S16) and the Grote-Hynes prediction (Eq. S14) to the simulation mean first-passage times $\tau_{\rm MFP}$, normalized by the neat water times $\tau^0_{\rm MFP}$, for the isomerization of butane and the inner dihedral of decane, plotted as a function of solvent viscosity.

## S11. BUTANE DIHEDRAL MEMORY KERNELS AND FITTING PARAMETERS

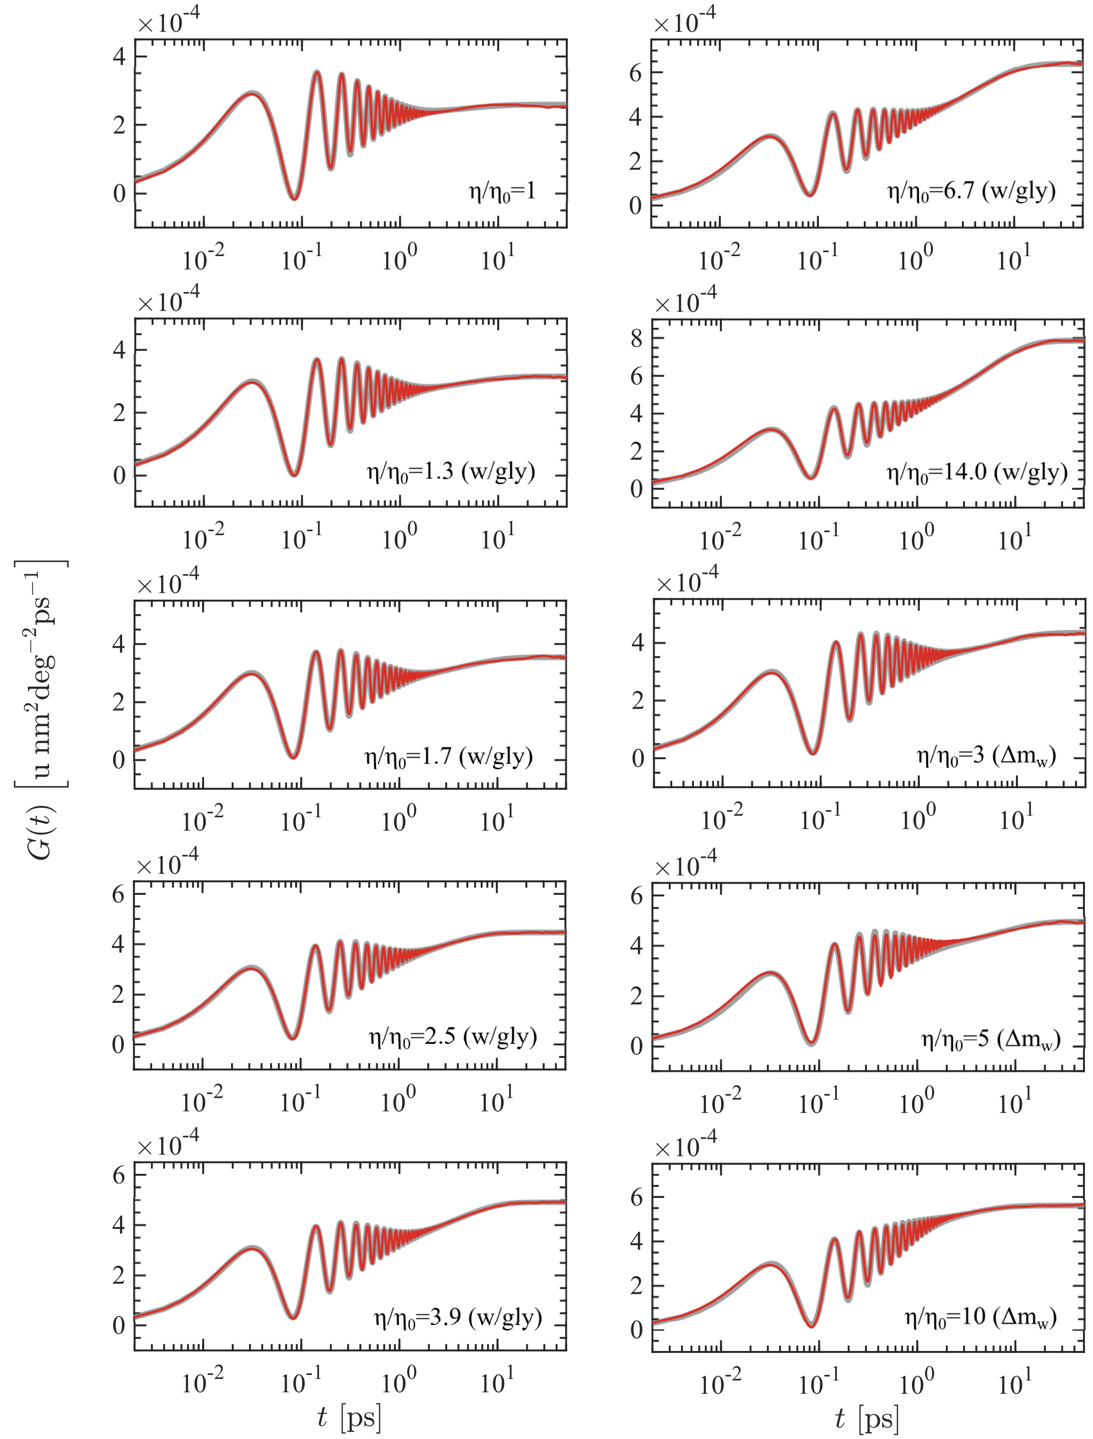


FIG. S14. The running integrals $G(t)$ associated with the memory kernels $\Gamma(t)$ for the butane dihedral for all solvent conditions. The red curves show $G(t)$ extracted from MD trajectories (see section S4). The thicker grey curve underlaid for each profile is the result for fitting Eq. S17 (Eq. 2 from the main text) to the MD results. Fitting is performed using non-linear least squares optimization.

In Fig. S14, we show the running integrals $G(t)$ of the memory kernels for the butane dihedral extracted from the MD trajectories under all solvent conditions. In Eq. 2 of the main manuscript, we propose a functional form for the the memory kernels $\Gamma(t)$ associated with the running integrals in Fig. S14. To fit to the extracted memory kernels, we fit the running integral form of the following series:

$$\Gamma(t) \approx \sum_{i=1}^{3} \frac{\gamma_i^{\exp}}{\tau_i^{\exp}} e^{-t/\tau_i^{\exp}} + \frac{(1+\omega_1\tau_1^{\mathrm{osc}})\gamma_1^{\mathrm{osc}}}{2\tau_1^{\mathrm{osc}}} e^{-t/\tau_1^{\mathrm{osc}}} \left[\cos(\omega_1 t) + \frac{\sin(\omega_1 t)}{\omega_1 \tau_1^{\mathrm{osc}}}\right], \tag{S17}$$

which is the same as Eq. 2 in the main text for $m = 3$ and $n = 1$. The resulting parameters from the 9-parameter fit in Eq. S17 are plotted in Fig. S15. These parameters are the same that appear in Fig. 3 in the main manuscript.

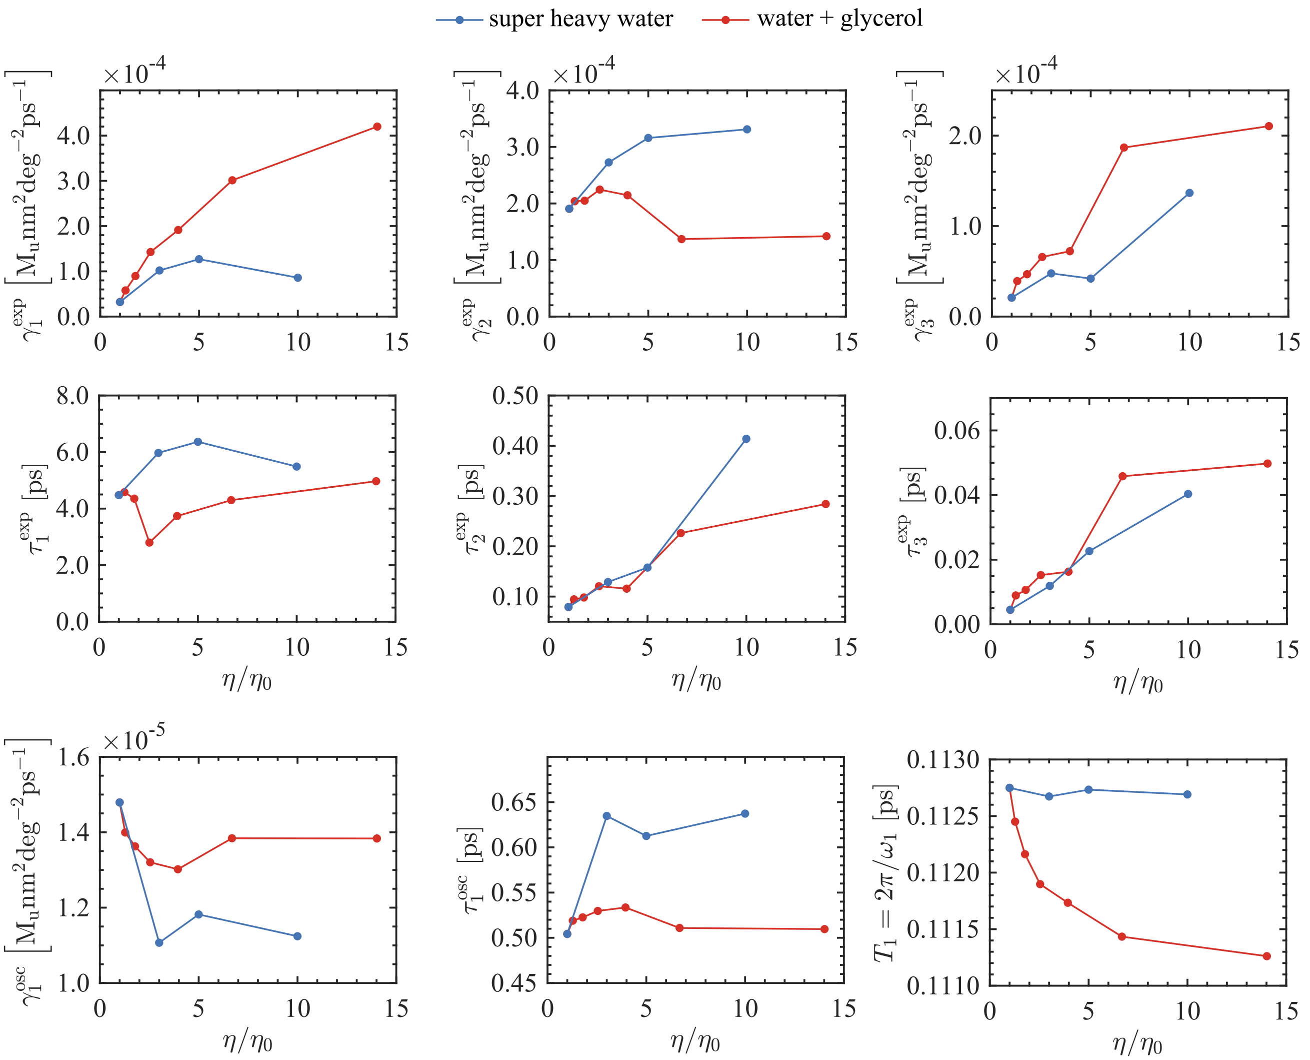


FIG. S15. Fitting parameters for memory kernels extracted from MD butane simulations plotted as a function of solvent viscosity. Comparison between super-heavy water solvent (blue) and aqueous-glycerol solvent (red). Fits are given by Eq. S17 and Eq. 2 in the main document, with m=3 and n=1, resulting in 9 fitting parameters for each kernel. $\gamma_i^{\exp}$ are the coefficients for the exponentially-decaying terms, and $\tau_i^{\exp}$ are the time scales, for $i = 1, 2, 3$. $\gamma_j^{\mathrm{osc}}$ is the coefficient for the single decaying-oscillating term, $T_1^{\mathrm{osc}}$ is the period of oscillation ($T_1^{\mathrm{osc}} = 2\pi/\omega_1$, as presented in the main text), and $\tau_1^{\mathrm{osc}}$ is the exponential time scale.

## S12. EFFECTS OF MEMORY KERNEL OSCILLATION ON GROTE-HYNES PREDICTIONS

In Fig. 4A of the main manuscript, we present the Grote-Hynes predictions for the mean first-passage times of butane and decane isomerization using memory kernels extracted from simulations. As evident in Figs. 2A and B of the main manuscript and Fig. S4, the memory kernels extracted for butane exhibit substantial contributions from oscillating modes. Our fitting results, obtained from Eq. 5 in the main text (and Eq. S17), indicate that only a single oscillating mode significantly contributes to the memory kernels. To evaluate the Grote-Hynes prediction, we numerically integrate the Laplace transform of the memory kernel to obtain the reactive frequency for the system, denoted as $\lambda$. To assess the influence of the oscillating mode on the Grote-Hynes prediction, we calculate the $\tau_{\mathrm{GH}}$ (Eq. 3 of the main text) for the extracted MD kernels of butane, the fully recombined fit of Eq. 5 from the main text including all three exponential terms and the single oscillating term (fit all), a partially recombined version of Eq. 5 consisting solely of the three exponential components (fit exponential), and solely the single oscillating component (fit oscillating). We present the results in Fig. S16. The Grote-Hynes predictions incorporating the extracted kernels and the fully recombined fits are in exact agreement. Upon removing the oscillating component, we observe an absolute decrease in the predicted times, but no impact on the scaling. This makes sense when we evaluate the predicted times associated with just the oscillating components, which are equal for all systems. Consequently, we can conclude that the pronounced oscillations observed in the butane memory kernels influence the absolute times in the Grote-Hynes predictions while leaving the viscosity-scaling unaffected.

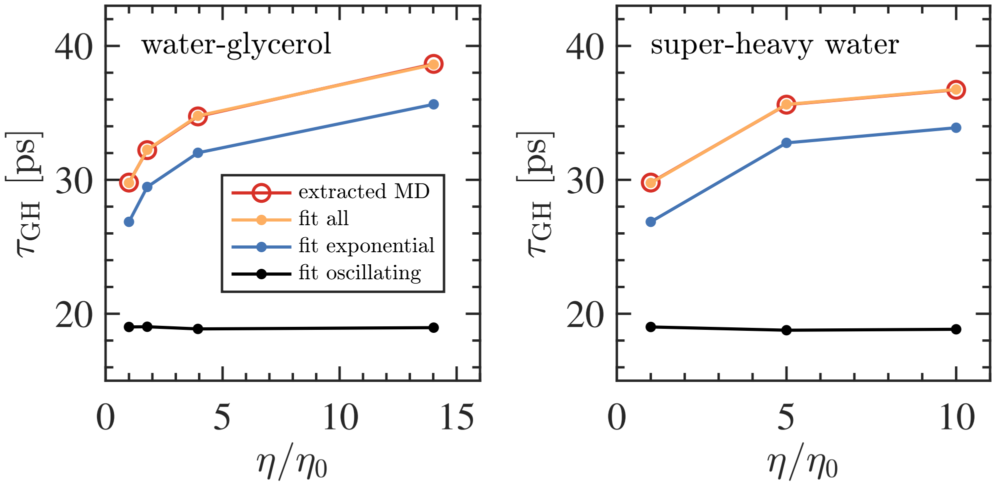


FIG. S16. Grote-Hynes predictions for butane isomerization times for systems with, and without, oscillating memory contributions. The extracted MD results are the same as shown in the main manuscript (Fig. 4A). The memory kernels are fit with Eq. 5 from the main text (also Eq. S17 of this SI). Using the fitting results, we reconstruct the full memory kernel (fit all), only the exponential contributions (fit exponential), and only the single oscillating contribution (fit oscillating), and hence evaluate the Grote-Hynes prediction $tau_{\mathrm{GH}}$ for each case. Results are shown for the water-glycerol mixtures, and the super-heavy water solvents.

[1] J. L. F. Abascal and C. Vega, The Journal of Chemical Physics **123**, 234505 (2005).
[2] C. Oostenbrink, A. Villa, A. E. Mark, and W. F. Van Gunsteren, Journal of Computational Chemistry **25**, 1656 (2004).
[3] J.-P. Ryckaert and A. Bellemans, Faraday Discussions of the Chemical Society **66**, 95 (1978).
[4] B. Hess, H. Bekker, H. J. C. Berendsen, and J. G. E. M. Fraaije, Journal of Computational Chemistry **18**, 1463 (1997).
[5] H. J. C. Berendsen, J. P. M. Postma, W. F. van Gunsteren, A. DiNola, and J. R. Haak, The Journal of Chemical Physics **81**, 3684 (1984).
[6] C. Ayaz, L. Scalfi, B. A. Dalton, and R. R. Netz, Physical Review E **105**, 54138 (2022).
[7] C. Ayaz, L. Tepper, F. N. Brünig, J. Kappler, J. O. Daldrop, and R. R. Netz, Proceedings of the National Academy of Sciences **118**, e2023856118 (2021).
[8] B. Kowalik, J. O. Daldrop, J. Kappler, J. C. F. Schulz, A. Schlaich, and R. R. Netz, Physical Review E **100**, 12126 (2019).
[9] J. O. Daldrop, J. Kappler, F. N. Brünig, and R. R. Netz, Proceedings of the National Academy of Sciences **115**, 5169 (2018).
[10] J.-P. Ryckaert, G. Ciccotti, and H. J. C. Berendsen, Journal of Computational Physics **23**, 327 (1977).
[11] R. F. Grote and J. T. Hynes, The Journal of Chemical Physics **73**, 2715 (1980).
